# Supplementary material for: Parallel Optimization of Polynomials for Large-scale Problems in Stability and Control
Source: arXiv:1702.05851 source file (2017-02-20)
Supplement: Supplementary file 1 [file appendix1.tex]

\chapter{RAW DATA}
